# Supplementary material for: Efficient Planning under Partial Observability with Unnormalized Q Functions and Spectral Learning
Source: arXiv:1911.05010 source file (2019-11-22)
Supplement: Supplementary file 1 [file appendix.tex]

\section{Proof for Lemma~\ref{matrix}}
\begin{proof}
We will show this by induction. 
First we need to show that:
$$\bm{\mu}^\top \mat{B}_{a_1o_1} =  \begin{bmatrix} 
                                        \Prob(S_2 = s^1, o_1, a_1) \\
                                        \vdots \\
                                        \Prob(S_2 = s^k, o_1,a_1)
                                    \end{bmatrix}^\top$$
\begin{align*}
    \bm{\mu}^\top \mat{B}_{a_1o_1}&= \begin{bmatrix} 
                                        \Prob(S_1 = s^1)  \\
                                        \vdots \\
                                        \Prob(S_1 = s^k)
                                    \end{bmatrix}^\top
                                    \begin{bmatrix}
                                    \Prob(A_1 = a_1|S_1 = s^1)&\cdots &0\\
                                    \vdots &\vdots &\vdots\\
                                    0&\cdots& \Prob(A_1 = a_1|S_1 = s^k)
                                    \end{bmatrix}\\
                                    &\begin{bmatrix}
                                    \Prob(S_2 = s^1|S_1 = s^1, A_1 = a_1) & \cdots &\Prob(S_2 = s^k|S_1 = s^1, A_1 = a_1)\\
                                    \vdots &\vdots &\vdots\\
                                     \Prob(S_2 = s^1|S_1 = s^k, A_1 = a_1) & \cdots &\Prob(S_2 = s^k|S_1 = s^k, A_1 = a_1)
                                    \end{bmatrix}\\
                                    &\begin{bmatrix}
                                    \Prob(O_1 = o_1|S_2 = s^1, A_1 = a_1)&\cdots &0\\
                                    \vdots&\vdots&\vdots\\
                                    0&\cdots&\Prob(O_1 = o_1|S_2 = s^k, A_1 = a_1)
                                    \end{bmatrix}\\
                                &= \begin{bmatrix} 
                                        \Prob(S_1 = s^1, A_1 = a_1)  \\
                                        \vdots \\
                                        \Prob(S_1 = s^k, A_1 = a_1)
                                    \end{bmatrix}^\top
                                    \begin{bmatrix}
                                    \Prob(S_2 = s^1|S_1 = s^1, A_1 = a_1) & \cdots &\Prob(S_2 = s^k|S_1 = s^1, A_1 = a_1)\\
                                    \vdots &\vdots &\vdots\\
                                     \Prob(S_2 = s^1|S_1 = s^k, A_1 = a_1) & \cdots &\Prob(S_2 = s^k|S_1 = s^k, A_1 = a_1)
                                    \end{bmatrix}\\
                                    &\begin{bmatrix}
                                    \Prob(O_1 = o_1|S_2 = s^1, A_1 = a_1)&\cdots &0\\
                                    \vdots&\vdots&\vdots\\
                                    0&\cdots&\Prob(O_1 = o_1|S_2 = s^k, A_1 = a_1)
                                    \end{bmatrix}\\
                                & = \begin{bmatrix} 
                                        \sum_s\Prob(S_2 = s^1, S_1 = s, A_1 = a_1)  \\
                                        \vdots \\
                                        \sum_s\Prob(S_2 = s^k, S_1 = s, A_1 = a_1)
                                    \end{bmatrix}^\top
                                    \begin{bmatrix}
                                    \Prob(O_1 = o_1|S_2 = s^1, A_1 = a_1)&\cdots &0\\
                                    \vdots&\vdots&\vdots\\
                                    0&\cdots&\Prob(O_1 = o_1|S_2 = s^k, A_1 = a_1)
                                    \end{bmatrix}\\
                                & = \begin{bmatrix} 
                                        \Prob(S_2 = s^1, A_1 = a_1) \Prob(O_1 = o_1|S_2 = s^1, A_1 = a_1) \\
                                        \vdots \\
                                        \Prob(S_2 = s^k, A_1 = a_1)\Prob(O_1 = o_1|S_2 = s^k, A_1 = a_1)
                                    \end{bmatrix}^\top\\
                                & = \begin{bmatrix} 
                                        \Prob(S_2 = s^1, O_1 = o_1, A_1 = a_1) \\
                                        \vdots \\
                                        \Prob(S_2 = s^k, O_1 = o_1, A_1 = a_1)
                                    \end{bmatrix}^\top 
\end{align*}
Then let us assume that:
$$\bm{\mu}^\top \mat{B}_{a_1o_1}\cdots \mat{B}_{a_{n-1}o_{n-1}} = \begin{bmatrix} 
                                        \Prob(S_{n} = s^1,  a_1o_1\cdots a_{n-1}o_{n-1}) \\
                                        \vdots \\
                                        \Prob(S_{n} = s^k,  a_1o_1\cdots a_{n-1}o_{n-1})
                                    \end{bmatrix}^\top$$
Then we have:
\begin{align*}
    \bm{\mu}^\top \mat{B}_{a_1o_1}\cdots \mat{B}_{a_{n}o_{n}} & = \begin{bmatrix} 
                                        \Prob(S_{n} = s^1,  a_1o_1\cdots a_{n-1}o_{n-1}) \\
                                        \vdots \\
                                        \Prob(S_{n} = s^k,  a_1o_1\cdots a_{n-1}o_{n-1})
                                    \end{bmatrix}^\top
                                    \begin{bmatrix}
                                    \Prob(A_n = a_n|S_n = s^1)&\cdots &0\\
                                    \vdots &\vdots &\vdots\\
                                    0&\cdots& \Prob(A_n = a_n|S_n = s^k)
                                    \end{bmatrix}\\
                                    &\begin{bmatrix}
                                    \Prob(S_{n+1} = s^1|S_n = s^1, A_n = a_1) & \cdots &\Prob(S_{n+1}= s^k|S_n = s^1, A_n = a_1)\\
                                    \vdots &\vdots &\vdots\\
                                     \Prob(S_{n+1} = s^1|S_n = s^k, A_n = a_1) & \cdots &\Prob(S_{n+1} = s^k|S_n = s^k, A_n = a_1)
                                    \end{bmatrix}\\
                                    &\begin{bmatrix}
                                    \Prob(O_n = o_n|S_n = s^1, A_n = a_n)&\cdots &0\\
                                    \vdots&\vdots&\vdots\\
                                    0&\cdots&\Prob(O_n = o_n|S_n = s^k, A_n = a_1)
                                    \end{bmatrix}\\
                                    & = \begin{bmatrix} 
                                        \Prob(S_{n+1} = s^1,  a_1o_1\cdots o_{n}a_{n}) \\
                                        \vdots \\
                                        \Prob(S_{n+1} = s^k,  a_1o_1\cdots o_{n}a_{n})
                                    \end{bmatrix}^\top
\end{align*}
\end{proof}

\begin{theorem}
Assume a WFA $A = \langle \bm{\alpha}, \{\mat{A}_{\sigma}\}_{\sigma \in \Sigma}, \mat{\Omega}\rangle$ realize the function $r(x)\Prob(x)$ for all $x \in \Sigma^*$ and the spectral radius $\rho(\sum_{\sigma \in \Sigma}\mat{A}_{\sigma}) < 1$. Then the WFA $B = \langle \bm{\alpha}_0, \mat{A}_{\sigma}, (\mat{I} - \sum_{\sigma\in \Sigma}\gamma\mat{A}_{\sigma})^{-1}\Omega \rangle$ realizes a function that is proportional to the function $Q$.
\end{theorem}
\begin{proof}
\begin{align*}
    Q(h, a, o) &= \Exp_{\ten{T}_\mat{\Pi}}(r_t + \gamma r_{t+1} + \gamma^2 r_{t+2} + \cdots |h, a, o)\\
    & = r(hao)\frac{\Prob(hao)}{\Prob(hao)} + \gamma \sum_{y_1 \in \Sigma}r(haoy_1)\frac{\Prob(haoy_1)}{\Prob(hao)} +\\  & ~~~~~~\gamma^2 \sum_{y_2\in \Sigma}\sum_{y_1 \in \Sigma}r(haoy_1y_2)\frac{\Prob(haoy_1y_2)}{\Prob(hao)}+\cdots\\
    &= \sum_{y\in \Sigma^*}\gamma^{|y|}r(haoy)\frac{\Prob(haoy)}{\Prob(hao)}\\
    &\propto \sum_{y\in \Sigma^*}\gamma^{|y|}r(haoy)\Prob(haoy)\\
    &= \sum_{y \in \Sigma^*}\gamma^{|y|}\bm{\alpha}_0^\top \mat{A}_{h}\mat{A}_{ao}\mat{A}_y\vec{\omega}\\
    &= \bm{\alpha}_0^\top \mat{A}_h\mat{A}_{ao}\sum_{y \in\Sigma^*}\gamma^{|y|}\mat{A}_y\vec{\omega}\\
    &= \bm{\alpha}_0^\top \mat{A}_h\mat{A}_{ao}(\mat{I} - \sum_{\sigma\in \Sigma}\gamma\mat{A}_{\sigma})^{-1}\vec{\omega}
\end{align*}
\end{proof}

\begin{lemma}
\label{matrix}
$$[\bm{\mu}^\top \mat{B}_{a_1o_1}\cdots \mat{B}_{a_To_T}]_i =\Prob(S_{n+1} = s^i, a_1o_1\cdots a_To_T)$$
\end{lemma}
Let $\Sigma = \mathcal{A}\times\mathcal{O}$, it is easy to show that given a trajectory $a_1o_1\cdots a_To_T$ sampled from a POMDP, the WFA $\langle \bm{\mu}, \{\mat{B}_{ao}\}_{ao \in \Sigma}, \bm{1}\rangle$ realize the probability distribution of the corresponding POMDP, i.e. we have the following lemma hold. 
\begin{lemma}
$\Prob(a_1o_1\cdots a_To_T) = \bm{\mu}^\top \mat{B}_{a_1o_1}\cdots \mat{B}_{a_To_T}\bm{1}$
\end{lemma}
\begin{proof}
By Lemma~\ref{matrix}, we have:
\begin{align*}
    \bm{\mu}^\top \mat{B}_{a_1o_1}\cdots \mat{B}_{a_To_T}\bm{1} & = \sum_s\Prob(S_{n+1} = s, a_1o_1\cdots a_To_T)\\
    & = \Prob(a_1o_1\cdots a_To_T)
\end{align*}
\end{proof}
Furthermore, we have the next lemma holds:
\begin{lemma} Let $\bm{q} = \mathrm{vec}(\mathrm{diag}\{\bm{\Pi}\mat{R}^\top\})$, we have 
$$\mathrm{\Tilde{R}}(a_1 o_1 \cdots a_To_T)\Prob(a_1o_1\cdots a_To_T) = \bm{\mu}^\top \mat{B}_{a_1o_1}\cdots \mat{B}_{a_To_T}\bm{q}$$
\end{lemma}
\begin{proof}
By Lemma~\ref{matrix}, it is easy to check that:
\begin{align*}
    \bm{\mu}^\top \mat{B}_{a_1o_1}\cdots \mat{B}_{a_To_T}\bm{q} &= \sum_a\sum_s r(s, a)\Prob( s, a| a_1o_1\cdots a_To_T)\\
    &~~~~~~\Prob(a_1o_1\cdots a_To_T)\\
    &= \Exp_{\ten{T}_\mat{\Pi}}(r(S, A)|a_1o_1\cdots a_To_T)\\
    &~~~~~~\Prob(a_1o_1\cdots a_To_T)\\
    &= \Tilde{r}(a_1o_1\cdots a_To_T)\Prob(a_1o_1\cdots a_To_T)
\end{align*}
\end{proof}
